# Supplementary material for: Direct imaging of molecular symmetry by coherent anti-Stokes Raman scattering
Source: arXiv:1511.04219 source file (2015-11-13)
Supplement: Supplementary file 1 [file Supplementary_Information.pdf]

# Supplementary Information

C. Cleff, A. Gasecka, P. Ferrand, H. Rigneault, S. Brasselet and J. Duboisset

## S1 - Connection between circular polarization and spherical harmonics

Vectors quantities (rank 1 tensor) can be expressed either in the Cartesian basis i=x,y,z or in spherical basis $Y_m^{l=1}$ with m=-1,0,1. The unitary transformation between the two bases is given by Table S1 [1].

| | x | y | z |
|---|---|---|---|
| $-\sqrt{4\pi/3}\,Y_1^1$ | $-1/\sqrt{2}$ | $-i/\sqrt{2}$ | |
| $-\sqrt{4\pi/3}\,Y_0^1$ | | | 1 |
| $-\sqrt{4\pi/3}\,Y_{-1}^1$ | $1/\sqrt{2}$ | $-i/\sqrt{2}$ | |

Table S1: Expression of $Y_m^{l=1}$ (m=1,0,-1) on the Cartesian basis

The electric fields expressed in the spherical basis write:

$$E_1^1 = -\frac{E_{0,\circlearrowleft}}{\sqrt{2}}(x + iy)$$

$$E_0^1 = E_{0,\nearrow}\,z$$

$$E_{-1}^1 = \frac{E_{0,\circlearrowright}}{\sqrt{2}}(x - iy),$$

where $E_{0,\circlearrowleft}$, $E_{0,\nearrow}$ and $E_{0,\circlearrowright}$ represent the norms of the electric field. These field vectors components coincide with the in-plane left circularly polarized field, axial and right circularly polarized fields, which are all invariant through rotations around z axis. In the spherical basis, and using table S1, these three polarization states can be written in terms of $Y_m^{l=1}$ with m=1,0,-1.

$$E_1^1 = E_{\circlearrowleft} = -\sqrt{4\pi/3}\,E_{0,\circlearrowleft}\,Y_1^1$$

$$E_0^1 = E_{\nearrow} = -\sqrt{4\pi/3}\,E_{0,\nearrow}\,Y_0^1$$

$$E_{-1}^1 = E_{\circlearrowright} = -\sqrt{4\pi/3}\,E_{0,\circlearrowright}\,Y_{-1}^1$$

with

$$Y_1^1(\theta,\varphi) = -\sqrt{3/8\pi}\,sin\theta e^{i\varphi}$$

$$Y_0^1(\theta,\varphi) = -\sqrt{3/4\pi}\,cos\theta$$

$$Y_{-1}^{1}(\theta,\varphi)=\sqrt{3/8\pi}\,sin\theta e^{-i\varphi}$$

Consequently, the product of four electric fields involved in the constitutive equation

$$E_{as}=\bar{\chi}^{(3)}.\left(\hat{e}^{*}{}_{as}\otimes\vec{E}_{p}\otimes\vec{E}^{*}{}_{s}\otimes\vec{E}_{pr}\right)$$

generates a field function $\bar{F}$

$$\bar{F}=\hat{e}^{*}{}_{as}\otimes\vec{E}_{p}\otimes\vec{E}^{*}{}_{s}\otimes\vec{E}_{pr}.$$

In the case of degenerated CARS, when pump and probe fields are equal, and considering in-plane circular polarization states only, the field function $\bar{F}$ can only exhibit rotational invariant symmetries of order 0, 2 or 4

$$F_{m_{\bar{F}}=0}(\theta,\varphi)=E_{1}^{1}E_{1}^{1*}E_{1}^{1}E_{1}^{1*}=E_{1}^{1}E_{-1}^{1}E_{1}^{1}E_{-1}^{1}\propto\sin\theta^{4}$$

$$F_{m_{\bar{F}}=2}(\theta,\varphi)=E_{1}^{1}E_{1}^{1*}E_{1}^{1}E_{-1}^{1}{}^{*}=E_{1}^{1}E_{-1}^{1}E_{1}^{1}E_{1}^{1}\propto\sin\theta^{4}\,e^{2i\varphi}$$

$$F_{m_{\bar{F}}=4}(\theta,\varphi)=E_{1}^{1}E_{-1}^{1}{}^{*}E_{1}^{1}E_{-1}^{1}{}^{*}=E_{1}^{1}E_{1}^{1}E_{1}^{1}E_{1}^{1}\propto\sin\theta^{4}\,e^{4i\varphi}$$

The spherical functions $F_{m_{\bar{F}}}$ are linked to the spherical harmonic function by the Clebch-Gordan coefficient according to [2]:

Order 0: $F_{m_{\bar{F}}=0}=\frac{1}{\sqrt{70}}Y_{0}^{4}-\frac{2}{\sqrt{63}}Y_{0}^{2}+\frac{2}{\sqrt{45}}Y_{0}^{0}$

Order 2: $F_{m_{\bar{F}}=2}=\frac{1}{\sqrt{28}}Y_{2}^{4}-\sqrt{\frac{3}{14}}Y_{2}^{2}$

Order 4: $F_{m_{\bar{F}}=4}=Y_{4}^{4}$

## S2- relation between Vibration symmetry and measured Orders

The spontaneous Raman active vibration modes of the cubic space group can be decomposed on the spherical harmonic basis, based on the irreducible representation described by [3].

$A_{1g}$ → $\bar{\alpha}_{m_F=0}$

$E_g$ → $\bar{\alpha}_{m_F=0}+\bar{\alpha}_{m_F=2}$

$T_{2g}$ → $\bar{\alpha}_{m_F=2}$

The Symmetry-resolved Raman spectrum shows the different symmetry orders of each resonance, see figure 1. The $A_{1g}$ resonance is mainly present on the order 0, the $T_{2g}$ is only present on the order 2 and the $E_g$ resonance is present on both order 0 and 2.

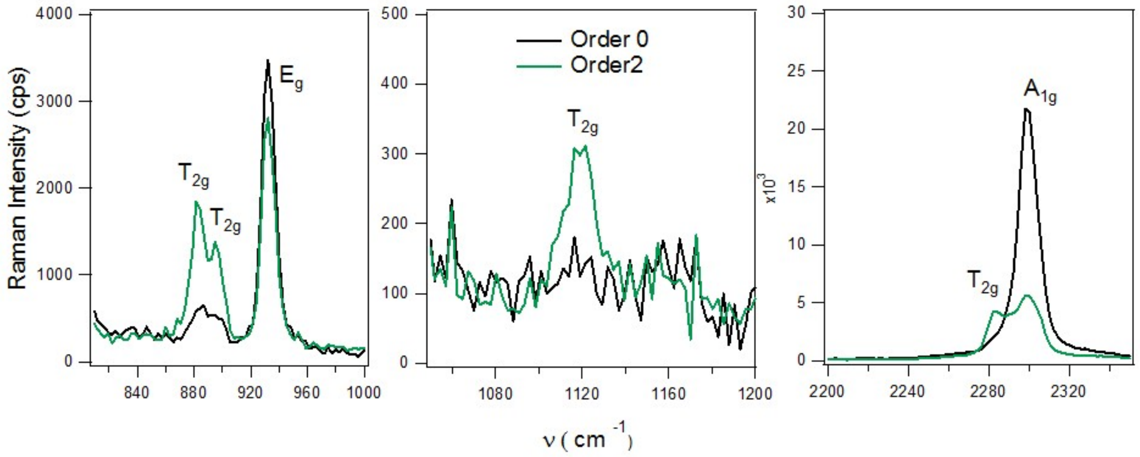


**Figure 1: Symmetry-resolved spontaneous Raman spectrum with the vibration assignments. The order 0 spectrum was recovered using left-hand circular polarization excitation and left-hand circular polarization detection. The order 2 spectrum was recovered using the same excitation and with a right-hand circular polarization.**

The nonlinear susceptibility $\chi^{(3)}$ involved in the CARS process can be written as a tensorial product of the Stokes susceptibility by the anti-Stokes susceptibility [4]

$$\bar{\chi}^{(3)} = \bar{\alpha}_{Stokes} \otimes \bar{\alpha}_{anti-Stokes}.$$

Using the spherical harmonic composition, the vibrational modes in CARS are decomposed along the orders

$A_{1g}$ → $\bar{\chi}_{m_F=0}$

$E_g$ → $\bar{\chi}_{m_F=0} + \bar{\chi}_{m_F=2} + \bar{\chi}_{m_F=4}$

$T_{2g}$ → $\bar{\chi}_{m_F=4}$

## S3 – Quantitative values on MLV

Following the CARS signal symmetry decomposition, the order 0 and order 2 images are weighted by the molecular density. In order to retrieve quantitative information about the molecular organization independently from this density, the order 2 image needs to be divided by the total intensity image. The square root of this ratio allows to scale with a normalized susceptibility, independent of the molecular density, see Fig 1 (a).  The average value of normalized order 2 on the MLV contour is 0.49 with a standard deviation of 0.06, see the histogram Fig 1 (b). This value is in good agreement with quantitative orders previously published in literature, based on more traditional linear polarization tuning [6].

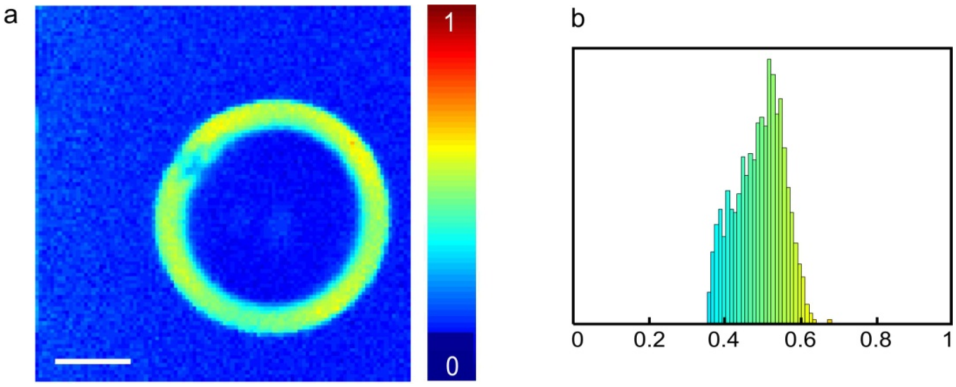


Figure 2: (a) square root of the ratio between order 2 and the total CARS intensity. (b) histogram of the ratio values of the MLV.

## M1 – Movie of Zeolite spectrum

Movie of regular CARS, order 0 and order 4 spectra. 88 images are taken while the Raman frequency was scanned from 778 to 1200 $cm^{-1}$and 36 images are taken from 2257 to 2347 $cm^{-1}$. Scale bar 10 µm.

## References

[1] Jerphagnon J., Chemla D., Bonneville R. The description of the physical properties of condensed matter using irreducible tensors. Advances in Physics, **27**, 609-650 (1978).

[2] Duboisset J., Rigneault H., Brasselet S. Filtering of matter symmetry properties by circularly polarized nonlinear optics. Physical Review A, **90**, 063827 (2014).

[3] Altmann S. L., Cracknell A. P. Lattice harmonics I. Cubic group. Reviews of modern physics, **37**, 19-32 (1965)

[4] Yuratich M. A., Hanna D. C. Coherent anti-stokes Raman spectroscopy (CARS) selection rules, depolarization ratios and rotational structure. Molecular Physics, **3**, 671-682 (1977)

[5] Marcolli C., Lainé P., Bühler R., Calzaferri G., Tomkinson J. Vibrations of H8Si8O12, D8Si8O12, and H10Si10O15 As Determined by INS, IR, and Raman Experiments. The Journal of Physical Chemistry B, **101**, 1171-1179 (1997)

[6] Bioud F.-Z., Gasecka P., Ferrand P., Rigneault H., Duboisset J. and Brasselet S. Structure of molecular packing probed by polarization-resolved nonlinear four-wave mixing and coherent anti-Stokes Raman-scattering microscopy. Phys Rev A, **89**, 013836 (2014).
